# Supplementary material for: Graph Transformer GANs with Graph Masked Modeling for Architectural Layout Generation
Source: arXiv:2401.07721 source file (2024-01-15)
Supplement: Supplementary file 1 [file 6appendix.tex]

This supplementary document provides additional details and results supporting the claims of the main paper.

\section{Limitations}

Although GTGAN can be applied to house layout and roof generation tasks separately, it is not yet ready to combine these two tasks to generate a fully automated house layout and roof design. 
In our future work, we will introduce a 3D house model to GTGAN to propose a unified framework to automatically generate a complete house design to help designers reduce the workload.
In addition, we will also introduce the user's interactive information to generate a more user-desired house structure.
Finally, GTGAN generates axis-aligned rectangles as rooms, but in real life, there can be exceptions to this, e.g., tilted or curvy walls, room extension at the exit, etc. In our future work, we will consider all of these, especially since they lead to overlaps between the axis-aligned room rectangles.
